# Supplementary material for: Kinetic theory of driven granular fluids
Source: arXiv:1803.10137 source file (2018-03-27)
Supplement: Supplementary file 1 [file AppendixJ.tex]

% Appendix Template

\chapter{Expressions from linear Grad's moments method at moderate densities} 

\label{AppendixJ} 

\lhead{Appendix J. \emph{Expressions from linear Grad's moments method at moderate densities}}

In terms of the traceless part of the (kinetic) pressure tensor $\Pi_{ij}=P_{ij}^k-nT \delta_{ij}$, the results can be written as

\beq
\label{3.49}
\Pi_{yy}^*=\Pi_{zz}^*=-\frac{2\gamma^*+g \zeta_0^*}{2\gamma^*+g \nu_\eta^*}, \quad \Pi_{xx}^*=-(d-1)\Pi_{yy}^*,
\eeq
\beq
\label{3.50}
\Pi_{xy}^*=-\frac{1+\Pi_{yy}^*-\frac{2^{d-2}}{d+2} \phi g  (1+\al)(3-\al)}{2\gamma^*+g \nu_\eta^*}a^*,
\eeq
where here $\Pi_{ij}^*\equiv P_{ij}^k/n T$,
\beq
\label{3.51}
\phi=\frac{\pi^{d/2}}{2^{d-1}d \Gamma\left(\frac{d}{2}\right)}n\sigma^d
\eeq
is the solid volume fraction and $g(\phi)$ is the pair correlation function. %In addition, $\zeta_0^*$ 
and $\nu_\eta^*\equiv \nu_\eta/\nu_0$. % where $\nu$ is given by Eq.\ \eqref{nu}. 
The (dimensionless) collisional contribution $P_{ij,c}^*\equiv P_{ij}^c/(nT)$ to the pressure tensor is given by \cite{G13}
\beq
\label{3.52}
P_{ij,c}^*=\left[1+2^{d-2}(1+\al)\phi g\right]\delta_{ij}+\frac{2^{d-1}}{d+2}(1+\al)\phi g \Pi_{ij}^* -\frac{2^{2d+1}d}{\pi (d+2)^2}\phi^2 g (1+\al) a_{ij}^*,
\eeq
where $a_{ij}^*\equiv a_{ij}/\nu_0$. The (dimensionless) shear rate $a^*$ is finally determined from the steady state condition \eqref{apH14}, namely,
\beq
\label{3.53}
a^*=-\frac{d}{2}\frac{2\gamma^*+\zeta_0^*}{\Pi_{xy}^*+P_{xy,c}^*}.
\eeq
In the case of hard spheres ($d=3$), Eqs.\ \eqref{3.49}, \eqref{3.50}, \eqref{3.52} and \eqref{3.53} are consistent with the results obtained by Sangani \emph{et al.} \cite{SMTK96} in the USF state by using Grad's solution to the Enskog equation \cite{JR85}.

In summary, Eqs.\ \eqref{3.49}, \eqref{3.50}, \eqref{3.52} and \eqref{3.53} provide the elements of the (reduced) pressure tensor $P_{ij}/(nT)$  and the (reduced) shear rate $a^*$ in terms of the coefficient of restitution $\al$, the (dimensionless) friction coefficient $\gamma^*$ and the solid volume fraction $\phi$.
